# Supplementary material for: A Hybrid Approach to Formal Verification of Higher-Order Masked Arithmetic Programs
Source: arXiv:2006.09171 source file (2020-06-16)
Supplement: Supplementary file 1 [file appendix.tex]

\section{Type Inference Rules for First-Order}
\label{sec:rule4first}

\begin{figure*}
	\centering
	\begin{tabular}{rrr}
		$\inference{\vdash x_1\star x_2:\tau & x\leftarrow x_2\star x_1} {\vdash x:\tau }[({\sc Com})]$
		&  $\inference{\vdash x':\tau & x\leftarrow \neg x'} {\vdash x:\tau}[({\sc Ide}$_1$)]$ \\ \vspace{1em}
		$\inference{\vdash x':\sid & x\leftarrow  x' \bullet x' }{\vdash x:\sid}[({\sc Ide}$_2$)]$
		& $\inference{x\leftarrow x' \diamond x'}{\vdash x:\sid}[({\sc Ide}$_3$)]$ \\ \vspace{1em}
		$\inference{\vdash x':\sdd & x\leftarrow x' \bowtie x'}{\vdash x:\sdd}[({\sc Ide}$_4$)]$
		&  $\inference{\vdash x_1:\rud & \vdash x_2:\rud & x\leftarrow x_1\circ x_2 \\ \Dom(\Expr(x_1))\setminus\RVar(\Expr(x_2))\neq \emptyset} {\vdash x:\sid}[({\sc Sid}$_{4}$)]$  \\  %\vspace{1em}
		$\inference{\vdash x_1:\sid &  \vdash x_2:\sid & x\leftarrow x_1\bullet x_2  \\ \RVar(\Expr(e_1))\cap\RVar(\Expr(e_2))= \emptyset} {\vdash x:\sid}[({\sc Sid}$_{5}$)]$
		&  $\inference{ \vdash x_1:\sdd & \vdash x_2:\rud & x\leftarrow x_1\circ x_2\\ \Dom(\Expr(x_2))\setminus\RVar(\Expr(x_1)) \neq \emptyset}  {\vdash x:\sdd }[({\sc Sdd})]$
	\end{tabular}
	\caption{Type inference rules, where  $\star\in\Op, \ \circ\in\{\wedge,\vee,\odot,\times\}$, $\bullet\in\Op^\ast$, $\bowtie\in\{\wedge,\vee\}$ and $\diamond\in \{\oplus,-\}$.}
	\label{tab:firstordersemrules}
\end{figure*}

Figure~\ref{tab:firstordersemrules} presents type inference rules for first-order security.
We denote by $\Op^\ast$ the set $\Op\cup\{\ll,\gg\}$.
Rule ({\sc Com}) captures the commutative law of operators $\star\in\Op$. % in our type inference system.
Rules ({\sc Ide}$_i$) for $i=1,2,3,4$ are straightforward.
Rule ({\sc Sid}$_{4}$) states that
$x$ has type $\sid$ if $x\leftarrow x_1\circ x_2$ for $\circ\in\{\wedge,\vee,\odot,\times\}$, both $x_1$ and $x_2$ have type $\rud$, and
$\Expr(x_1)$ has a dominant variable $r$ which is not used by $\Expr(x_2)$.
Indeed, $\Expr(x)$ can be seen as $r\circ \Expr(x_2)$.
Rule ({\sc Sid}$_{5}$) states that expression
$x$ has type $\sid$ if $x\leftarrow x_1\bullet x_2$ for $\bullet\in\Op^\ast$,
both $x_1$ and $x_2$ have type $\sid$ (as well as its subtype $\rud$), and
the sets of random variables used by $\Expr(x_1)$ and $\Expr(x_2)$ are disjoint.
Indeed, for each valuation $\eta\in\Theta$, the distributions $\sem{x_1}_{\eta}$
and $\sem{x_2}_{\eta}$ are independent.
Rule ({\sc Sdd}) states that the variable $x$ has type $\sdd$ if $x\leftarrow x_1\circ x_2$ for $\circ\in\{\wedge,\vee,\odot,\times\}$,
$x_1$ has type $\sdd$, $x_2$ has type $\rud$, and
$\Expr(x_2)$ has a dominant variable $r$ which is not used by $\Expr(x_1)$.
Intuitively, $\Expr(x)$ can be safely seen as $\Expr(x_1)\circ r$.
